# Supplementary material for: Statics and Dynamics of Space-Charge-Layers in Polarized Inorganic Solid Electrolytes
Source: arXiv:2101.10294 source file (2021-01-25)
Supplement: Supplementary file 1 [file supporting_information.pdf]

# Electronic Supporting Information: Statics and Dynamics of Space-Charge Layers in Polarized Inorganic Solid Electrolytes

Katharina Becker-Steinberger[1, 2], Simon Schardt[3], Birger Horstmann[1, 2, 4], and Arnulf Latz[1,2, 4]

[1]*Helmholtz Institute Ulm (HIU), Helmholtzstraße 11, 89081 Ulm, Germany.*
[2]*Institute of Engineering Thermodynamics, German Aerospace Center (DLR), Pfaffenwaldring 38-40, 70569 Stuttgart, Germany.*
[3]*University of Würzburg, Campus Hubland Nord 32, 97074 Würzburg, Germany.*
[4]*Ulm University, Albert-Einstein-Alle 47, 89081 Ulm, Germany.*

January 25, 2021

## SI-1 Mathematical Model

### SI-1.1 Model Assumptions

For the sake of clarity, we summarize our basic assumptions regarding setup, domain geometry, interfaces, material composition and modeling, as well as processes and time scales.

**Setup and Geometry**

**SI-S1** Following the *polarization experiments*[1–3], we limit ourselves to modeling *SEs between two ion-blocking electrodes* which are connected to a high resistance voltage source.

**SI-S2** We investigate SEs with *perfectly planar and spatially fixed boundaries* and represent them in our simulations by 1D domains. The positive-electrode-SE interface and the negative-electrode-SE interface are denoted $\Gamma_\mathrm{C} = \{0\}$ and $\Gamma_\mathrm{A} = \{L_\mathrm{SE}\}$, respectively. There is *no loss of contact* between the phases.

**Material Composition and Properties**

**SI-M1** We model these SEs as *three component systems* consisting of mobile cations (indexed $+$), an immobile, negative charged background lattice (indexed 0) and vacant generalized cation sites (indexed $v$). The properties of the constituents are characterized by their molar masses $M_\alpha$, charge numbers $z_\alpha$, velocity fields $\mathbf{v}^\#_\alpha$ measured in a lab frame, and molar volumes $v_\alpha$, where $M_0$ is the molar mass of the total anion lattice backbone. Vacancies are considered to be mass- and chargeless, i.e., $M_v = z_v = 0$ and the anions are resting in the background lattice.

**SI-M2** We consider *incompressible, isotropic linear elastic, linear dielectric* crystalline SEs, i.e., the deformations of the ionic lattice are neglected. Technically, the incompressibility is ensured

by the limit $K_{\mathrm{SE}} \to \infty$, where $K_{\mathrm{SE}}$ is the bulk modulus. Since the anions are fixed to the background lattice, this implies that the anions do not have a velocity, i.e., $\mathbf{v}_0^{\#} = \mathbf{0}$.

**SI-M3** We assume that only the fixed background lattice is polarizable.

**SI-M4** Due to the production process, the SE may be inhomogeneous.

**Time Scales and Processes**

**SI-P1** We assume *isothermal conditions* at a constant temperature $\theta$.

**SI-P2** We consider time scales for changes in electric fields on which magnetic effects can be neglected (see e.g.,[4]).

**SI-P3** Elastic mechanical relaxations on the time scale of sound propagation are neglected i.e. *mechanical equilibrium* holds for the time scale of diffusion and internal mass convection. This implies a quasi-static force balance, in which convective momentum flux as well as mass accelerations are neglected.

**SI-P4** *Heterogeneous side reactions* at the electrodes are neglected. As a consequence SEs are charged only through the bulk and the non-linear processes in the SEs are not masked by other phenomena.

## SI-1.2 Incompressible Solid Electrolyte Model

This section includes some complementary aspects of the model derivation in Sec. 2.2.

### SI-1.2.1 Reference Frame

For consistency with Braun et al.[5], the transport theory is discussed relative to the center-of-mass velocity of the SE. The internal center-of-mass frame is the usual frame of reference to describe transport processes in liquid electrolytes. In contrast to that, the lab frame is a global frame of reference in which experimental measure are performed. The more common frame of reference to describe transport in solids is a lattice-fixed frame, see e.g.,[6]. Since we assume that the anions are resting in the background lattice (see assumption (SI-M1)), lattice-fixed coordinates corresponds to a Hitthorf frame, or $N$-th component frame[7], in which the $N$-th species—the anions—does not actively participate in the transport process. Furthermore, as (by assumption (SI-M2)) the lattice does not deform, this frame coincides with the lab frame. Subsequently, any quantity or parameter that is directly associated with the lattice frame is marked with superscript #.

The molar fluxes relative to the lattice, respectively, relative to the center-of-mass motion are given by

$$\mathbf{N}_\alpha^{\#} = c_\alpha \mathbf{v}_\alpha^{\#}, \qquad \alpha \in \{+, v\}, \tag{SI-1a}$$

$$\mathbf{N}_\alpha = c_\alpha \left(\mathbf{v}_\alpha^{\#} - \mathbf{v}\right), \qquad \alpha \in \{+, v, 0\}, \tag{SI-1b}$$

where $\mathbf{v}_\alpha^{\#}$ is the mean velocity of the $\alpha$-th species in a lab frame and $\mathbf{v}$ is the center-of-mass velocity, which mass averages the individual constituent velocities. Because of the immobility of the anion

background lattice, it is proportional to the cation velocity

$$\mathbf{v} = \frac{\rho_+ \mathbf{v}_+^\# + \rho_0 \mathbf{v}_0^\#}{\rho} = \frac{\rho_+}{\rho} \mathbf{v}_+^\#. \tag{SI-2}$$

Since the anions are resting in the lab frame, the center-of-mass velocity, the cation velocity and cation diffusion flux are proportional to each other. The mass diffusion flux of anions is compensated by their mass convective motion

$$\mathbf{N}_+ = c_+ \left(\mathbf{v}_+^\# - \mathbf{v}\right) = c_+ \frac{\rho_0}{\rho} \mathbf{v}_+^\# = c_+ \frac{\rho_0}{\rho_+} \mathbf{v}, \tag{SI-3a}$$

$$\mathbf{N}_0 = c_0 \left(\mathbf{v}_0^\# - \mathbf{v}\right) = -c_0.\mathbf{v} \tag{SI-3b}$$

Under the assumptions made in this work, in a lattice-fixed frame there are from the beginning only two independent fluxes, see Eq. (SI-1a). In each reference system the number of independent flows reduces by one. In a center-of-mass frame the fluxes of the anions and cations satisfy the side condition of mass conservation

$$\mathbf{N}_0 = -m_+ \mathbf{N}_+, \tag{SI-4}$$

which is used to "eliminate" the anion species. Thereby, $m_+ := M_+/M_0$ abbreviates the ratio of molar masses.

### SI-1.2.2 Transformation of Fluxes and Forces

In the main document, in Sec. 2.2.4, the entropy inequality is evaluated in a center-of-mass frame. Utilizing the mass conservation constraint (SI-4) gives that there are two independent fluxes, $\mathbf{N}_+, \mathbf{N}_v$, and two independent driving forces, $\tilde{\mathbf{X}}_+ := \mathbf{X}_+ - m_+ \mathbf{X}_0$, $\tilde{\mathbf{X}}_v := \mathbf{X}_v$, relative to the center-of-mass motion such that the entropy inequality and the Onsager relations are satisfied. Here $\mathbf{X}_\alpha = -(\nabla \mu_\alpha + z_\alpha F \nabla \phi), \alpha \in \{+,0\}$, denote the negative electrochemical potential gradients of ions and $\mathbf{X}_v = -\nabla \mu_v$ the negative chemical potential gradient of vacancies.

The entropy principle can also be evaluated in a lattice fixed reference system. Instead we transform here, for the sake of simplicity, only the fluxes and their conjugate driving forces. With regard to thermodynamic consistency, both the fluxes and the forces must be transformed in such a way that the entropy inequality and the Onsager relations are still fulfilled. The transformation between the fluxes is a simple consequence of their definition

$$\mathbf{N}_+^\# = \frac{\rho}{\rho_0} \mathbf{N}_+, \tag{SI-5a}$$

$$\mathbf{N}_v^\# = \mathbf{N}_v + \frac{c_v}{c_+} \frac{\rho_+}{\rho_0} \mathbf{N}_+. \tag{SI-5b}$$

Thus, introducing the vectors of independent fluxes $\mathbf{N}^\# := (\mathbf{N}_+^\#, \mathbf{N}_v^\#)^T$ and $\mathbf{N} := (\mathbf{N}_+, \mathbf{N}_v)^T$ they are

related by the linear transformation

$$\mathbf{N}^{\#} = \mathbf{A}\mathbf{N} \qquad \text{with } \mathbf{A} := \begin{pmatrix} \frac{\rho}{\rho_0} & 0 \\ 1 & \frac{c_v}{c_+}\frac{\rho_+}{\rho_0} \end{pmatrix}. \tag{SI-6}$$

Analogeously, we define the vectors of driving forces $\tilde{\mathbf{X}}^{\#} = (\tilde{\mathbf{X}}^{\#}_{+}, \tilde{\mathbf{X}}^{\#}_{v})^T$ and $\tilde{\mathbf{X}} = (\tilde{\mathbf{X}}_{+}, \tilde{\mathbf{X}}_{v})^T$. Then, the transformed driving force vector is given by

$$\tilde{\mathbf{X}}^{\#} = \mathbf{A}^{-T}\tilde{\mathbf{X}} \tag{SI-7}$$

and the entropy production due to diffusion reads

$$\zeta_{\text{diff}} = \tilde{\mathbf{X}} \cdot \mathbf{N} = \tilde{\mathbf{X}}^{\#} \cdot \mathbf{N}^{\#}. \tag{SI-8}$$

Furthermore, the fluxes have the suitable phenomenological representation

$$\mathbf{N}^{\#} = \mathbf{A}\mathbf{N} = \mathbf{A}\mathscr{L}\tilde{\mathbf{X}} = \mathbf{A}\mathscr{L}\mathbf{A}^T\tilde{\mathbf{X}}^{\#} = \mathscr{L}^{\#}\tilde{\mathbf{X}}^{\#}, \tag{SI-9}$$

where $\mathscr{L}^{\#} := \mathbf{A}\mathscr{L}\mathbf{A}^T$ denotes the Onsager matrix in a lattice-fixed frame, which automatically obeys Onsager's conditions.

#### SI-1.2.3 Duality Condition

It is clear that in an incompressible solids, each jump of an ion corresponds to a vacancy moving in the opposite direction; consequently, in a three-component system with one lattice fixed component, there is only one driving force and one flux. However, the form of this driving force is not a priori known. To the best of our knowledge this was first shown in Braun et al.[5] by deriving an additional side condition—a relation between the cation and the defect diffusion flux—from the time independence of $c_1$. The argumentation to derive this duality side condition is as follows.

Summing up the balance equations leads the balance equation for the conduction pathway sites

$$\partial_t(c_+ + c_v) + \nabla \cdot \left(\mathbf{N}^{\#}_{+} + \mathbf{N}^{\#}_{v}\right) = 0. \tag{SI-10}$$

In equilibrium it holds

$$\nabla \cdot \left(\mathbf{N}^{\#}_{+} + \mathbf{N}^{\#}_{v}\right) = 0. \tag{SI-11}$$

The sum of the lab frame fluxes can be related to the sum of center-of-mass fluxes utilizing relation (SI-3b) between anion flux relative to the center-of-mass motion and the center-of-mass velocity

and, then, using the mass conservation side condition (SI-4) to eliminate the anion flux

$$\begin{aligned}\mathbf{N}_+^\# + \mathbf{N}_v^\# &= \sum_{\alpha \in \{+,v\}} c_\alpha \left(\mathbf{v}_\alpha^\# - \mathbf{v}\right) + c_1 \mathbf{v} \\ &= \mathbf{N}_+ + \mathbf{N}_v - \frac{c_1}{c_0}\mathbf{N}_0 \\ &= \left(1 + m_+ \frac{c_1}{c_0}\right)\mathbf{N}_+ + \mathbf{N}_v\end{aligned} \tag{SI-12}$$

We abbreviate the composition dependent factor relating the center-of-mass fluxes by

$$\beta = \beta(c_1) := 1 + m_+ \frac{c_1}{c_0} = 1 + \frac{\rho_+}{\rho_0} + \frac{M_+ c_v}{\rho_0}. \tag{SI-13}$$

As can be seen from the first line in (SI-12), this coefficient is unity in a lattice fixed frame. Thus, there exists a vector potential $\mathbf{k}$ such that

$$\nabla \times \mathbf{k} = \mathbf{N}_v + \beta \mathbf{N}_+ = \mathbf{N}_v^\# + \mathbf{N}_+^\# \tag{SI-14}$$

Since, in equilibrium, all fluxes must vanish simultaneously, we can argue that $\mathbf{k} = \mathbf{0}$. We obtain the duality condition an a lattice fixed frame, respectively, a center-of-mass frame

$$\mathbf{N}_v^\# = -\mathbf{N}_+^\#, \tag{SI-15a}$$

$$\mathbf{N}_v = -\beta \mathbf{N}_+. \tag{SI-15b}$$

From condition (SI-15a) it follows that, the duality side condition complies with a relation between the cation and cation site velocity

$$\mathbf{v}_v^\# = \frac{c_+}{c_v}\mathbf{v}_+^\#. \tag{SI-16}$$

#### SI-1.2.4 Cation Flux and Baro-Diffusion Coefficient

In Sec. 2.2.6 of the main part, the driving force contributions are analyzed qualitatively. By decomposing the driving force into its contributions, the cation flux splits into contributions due to concentration gradients, pressure gradients, potential gradients as well as inhomogeneities

$$\mathbf{N}_+ = -\left(D_+ \nabla c_+ + D_{\text{ih}} \nabla c_1 + D_p \nabla p + b_+ \nabla \phi\right). \tag{SI-17}$$

Thereby, $D_+$ denotes the chemical diffusion coefficient, $D_p$ the baro-diffusion coefficient, $b_+$ the electrical cation mobility, and the parameter $D_{\text{ih}}$ quantifies the deviation from homogeneous equilibrium distributions of cations. Here we are particularly interested in gaining a better understanding of the baro-diffusion coefficient

$$D_p = \mathscr{L}_{++}\left(v_+ - m_+ v_0 - \beta v_v\right) \tag{SI-18}$$

by suitable reformulation. The thermodynamic constraint $\sum_{\alpha\in\{+,v,0\}} v_\alpha c_\alpha = 1$ allows $v_0$ to be expressed by the partial molar volumes of the cations and the cation sites. Along with elmentary transformations this leads to

$$\begin{aligned} D_p &= \mathscr{L}_{++}\left(v_+\frac{M_+}{M_0}\left(\frac{1}{c_0}-\frac{c_v}{c_0}v_v-\frac{c_+}{c_0}v_+\right)-\left(1+\frac{M_+}{M_0}\frac{c_1}{c_0}\right)v_v\right) \\ &= \mathscr{L}_{++}\left(-\frac{M_+}{\rho_0}\left(1+\frac{\rho_+}{\rho_0}\right)\Delta v\right) \\ &= \mathscr{L}_{++}\left(-\frac{M_+}{\rho_0}+\frac{\rho}{\rho_0}\Delta v\right) \\ &= -\mathscr{L}_{++}\frac{M_+}{\rho_0}\left(1-\frac{\rho}{M_+}\Delta v\right), \end{aligned} \tag{SI-19}$$

where $\Delta v := v_+ - v_v$ is the difference in cation and cation site partial molar volumes . Thus, the baro-diffusion coefficient is given by Eq. (22), which states that in incompressible SEs without lattice deformations, baro-diffusion is mainly caused by the inhomogeneity on the conduction pathway quantified by $\Delta v$.

### SI-1.2.5 Material Model

The material models considered in this work relies on a free energy function consisting of a reference free energy density, the free energy density due to the entropy of mixing $\rho\psi^{\mathrm{mix}}$, the mechanical free energy density $\rho\psi^{\mathrm{mech}}$, and the free energy due to polarization $\rho\psi^{\mathrm{P}}$. We model incompressible isotropic linear elastic, linear dielectric inorganic SEs (see assumption (SI-M2)). In this conceptional study, all contributions of free energy density are essentially chosen as in the previous work[5]:

$$\rho\psi^{\mathrm{mix}} = R\theta\left(c_+\ln\left(\frac{c_+}{c_1}\right)+c_v\ln\left(\frac{c_v}{c_1}\right)\right), \tag{SI-20}$$

$$\rho\psi^{\mathrm{mech}} = (K_{\mathrm{SE}}-p^\circ)\left(1-\frac{c}{c^\circ}h(c_+,c_v,c_0)\right)+K_{\mathrm{SE}}\frac{c}{c^\circ}h(c_+,c_v,c_0)\ln\left(\frac{c}{c^\circ}h(c_+,c_v,c_0)\right) \tag{SI-21}$$

$$\rho\psi^{\mathrm{P}} = -\frac{\varepsilon_{\mathrm{SE}}}{2}|\mathbf{E}|^2. \tag{SI-22}$$

Here $R$ and $\theta$ are the universal gas constant and the absolute temperature, $K_{\mathrm{SE}}$ denotes the bulk modulus, $\varepsilon_{\mathrm{SE}}$ the dielectric permittivity, and $c^\circ$ the reference summary concentration at reference pressure $p^\circ$. To account for size effects in this work without deviating too far from the original model[5], we modify the mechanical part of the free energy density slightly by introducing a function $h(c_+,c_v,c_0)$ characterizes an isotropic volumetric expansion due to local concentration variations. Similar modifications have also been made in models for liquid electrolytes, see e.g.,[8]. The elastic pressure as function of the volume is then given by linear elastic relation

$$p = p^\circ + K_{\mathrm{SE}}\left(\frac{c}{c^\circ}h(c_+,c_v,c_0)-1\right). \tag{SI-23}$$

In the incompressible limit of diverging bulk modulus, the chemical potentials derived from the

generalized material model take the form

$$\mu_\alpha = \mu_\alpha^\circ + v_\alpha(p - p^\circ) + R\theta \ln \frac{c_\alpha}{c_1}, \tag{SI-24a}$$

$$\mu_0 = \mu_0^\circ + v_\alpha(p - p^\circ), \tag{SI-24b}$$

where $\alpha \in \{+, v\}$ indicate the cations and the cation sites and $v_\alpha, \alpha \in \{0, +, v\}$, denote the partial molar volumes. For homogeneous distributions on the conduction pathway, i.e., $v_\alpha = 1/c^\circ$, the chemical potentials (SI-24a), (SI-24b) are equivalent to the ones derived by Braun et al.[5], where the lattice was assumed to be an equidistant grid.

### SI-1.3 Model Equations in Mechanical Equilibrium

To justify the assumption of mechanical equilibrium, we first reveal the scales in the momentum equation by dimensional analysis. In addition to the main part of this work, the driving force in mechanical equilibrium is explicitly written down and its transformation into the lattice fixed frame is specified.

#### SI-1.3.1 Quasi-Static Approximation of Momentum Conservation

We aim to compare the speed of the mechanical processes induced by polarization with other processes. Therefore, we choose a reference mean velocity

$$\mathrm{v}^R = L^R/t^R \quad \text{with} \quad L^R = L_{\text{diff}} = \sqrt{D_+^t t^R} \quad \text{and} \quad t^R \tag{SI-25}$$

being the diffusion length and time scale of the studied process (charge, discharge of cell or double layer). On the other hand we select as reference pressure $p^R$ the scale of the Maxwell pressure $p^R = \varepsilon_{\text{SE}}(U/L_{\text{diff}})^2$ at reference potential $\phi^R = U$, which is equal to the applied potential difference. The corresponding scale of the induced free charge density is $q_F^R = \varepsilon_{\text{SE}} U/L_{\text{diff}}^2$. The dimensionless formulation of the momentum equation (35) resulting from this scaling reads

$$\delta\left(\partial_{t^\star}\rho^\star \mathbf{v}^\star + \nabla\cdot(\rho^\star \mathbf{v}^\star \otimes \mathbf{v}^\star)\right) + \nabla p^\star + q_F^\star \nabla\phi^\star = 0, \tag{SI-26}$$

where dimensionless variables are labeled with an asterisk. The time scale of the studied process drops out and the dynamic contribution in Eq. (SI-26) scales with the factor $\delta = \rho^R (D_+^t)^2/(\varepsilon_{\text{SE}} U^2)$, which is very small even for diffusion constants of order $10^{-6}$ cm$^2$/s (of order $10^{-5}$). As a result, we can neglect dynamic and convective contributions in (SI-26) and obtain a quasi-static relation for the pressure gradients

$$\nabla p = -q_F \nabla\phi. \tag{SI-27}$$

#### SI-1.3.2 Driving Force

In mechanical equilibrium the elastic pressure is a dependent quantity determined up to a constant by the force balance (SI-27). This coupling of the elastic and the electrostatic forces allows us to eliminate one degree of freedom and to rewrite the chemical potential gradients of mobile species

(20) to

$$\nabla\mu_\alpha = \frac{\partial \mu_\alpha}{\partial c_+}\nabla c_+ + \frac{\partial \mu_\alpha}{\partial c_1}\nabla c_1 - \nu_\alpha q_F \nabla\phi. \tag{SI-28}$$

Hence, it leads to a dependence of the chemical potential gradients on the Coulomb force density. With Poisson's equation (38) this electrostatic force in Eq. (SI-28) can be replaced by a second order polynomial of the potential gradient. Thus, on time scales relevant for battery applications, the effective driving force (15) becomes

$$\begin{aligned}\overline{\mathbf{X}} &= \left(\frac{\partial \mu_+}{\partial c_+} - \beta\frac{\partial \mu_v}{\partial c_+}\right)\nabla c_+ + \left(\frac{\partial \mu_+}{\partial c_1} - \beta\frac{\partial \mu_v}{\partial c_1}\right)\nabla c_1 - \frac{M_+}{\rho_0}\left(1-\frac{\rho}{M_+}\Delta\nu\right) q_F\nabla\phi + F\overline{z}\nabla\phi \\ &= \left(\frac{\partial \mu_+}{\partial c_+} - \beta\frac{\partial \mu_v}{\partial c_+}\right)\nabla c_+ + \left(\frac{\partial \mu_+}{\partial c_1} - \beta\frac{\partial \mu_v}{\partial c_1}\right)\nabla c_1 + \left(\frac{M_+}{\rho_0}\left(1-\frac{\rho}{M_+}\Delta\nu\right)\nabla\cdot(\varepsilon_{\mathrm{SE}}\nabla\phi) + F\overline{z}\right)\nabla\phi \\ &:= \hat{\mathbf{X}}\end{aligned} \tag{SI-29}$$

In this work, any quantity in mechanical equilibrium is indicated by a hat.

### SI-1.3.3 Drift-Diffusion Flux and Transport Coefficients

By introducing a free charge dependent cation conductivity $\hat{\sigma}^\#$, the cation flux (25), respectively, (SI-17) in mechanical equilibrium can expressed in a form analogous to classical approaches

$$\hat{\mathbf{N}}_+ = -\left(D_+\nabla c_+ + D_{\mathrm{ih}}\nabla c_1 + \frac{\hat{\sigma}^\#}{z_+F}\frac{\rho_0}{\rho}\nabla\phi\right) \tag{SI-30}$$

Thereby, the conductivity is defined as

$$\hat{\sigma}^\# := z_+F\frac{\rho}{\rho_0}\left(b_+ - D_p q_F\right). \tag{SI-31}$$

Like the baro-diffusion coefficient we formulate the conductivity in terms of the inhomogeneity of the conduction pathways $\Delta\nu$. Inserting the cation mobility (32), the baro-diffusivity (33) and using $z_+ = -z_0$ and $M = M_+ + M_0$ yields

$$\begin{aligned}\hat{\sigma}^\# &= z_+F\frac{\rho}{\rho_0}\mathscr{L}_{++}\left(\frac{Mc_0}{\rho_0}z_+F + \frac{M_+}{\rho_0}\left(1-\frac{\rho}{M_+}\Delta\nu\right)F(z_+c_+ + z_0c_0)\right) \\ &= (z_+F)^2\frac{\rho}{\rho_0}\mathscr{L}_{++}\left(\frac{(M_+ + M_0)c_0}{\rho_0} + \frac{M_+}{\rho_0}\left(1-\frac{\rho}{M_+}\Delta\nu\right)(c_+ - c_0)\right) \\ &= (z_+F)^2\left(\frac{\rho}{\rho_0}\right)^2\mathscr{L}_{++}(1-(c_+ - c_0)\Delta\nu)\end{aligned} \tag{SI-32}$$

Utilizing the transformed cation mobility

$$\mathscr{L}^\#_{++} = \left(\frac{\rho}{\rho_0}\right)^2\mathscr{L}_{++} \tag{SI-33}$$

**Table SI-1** Material parameters for LLTO perovskite, LATP NaSICON, and amorphous LIPON as reported in literature[9–15] or calculated (indicated by ∗).

| Parameter | Value in LLTO | Ref. | Value in LATP | Ref. | Value in LIPON | Ref. | Unit |
|---|---|---|---|---|---|---|---|
| $\rho$ | 4.00 | Ref.[10] | 2.82 | Ref.[11] | 2.30 | | g/cm$^3$ |
| $M$ | 168.822 | * | 383.398 | * | 85.913 | * | g/mol |
| $\chi_{\mathrm{SE}}(\omega=\infty)$ | (90 | Ref.[12]) | 15 | Ref.[14] | 19.98 | Ref.[13] | - |
| $\chi_{\mathrm{SE}}(\omega=0)$ | $10^{05}$ | Ref.[12] | $1\times10^{03}$ | Refs.[12,14] | ($10^{05}$ | Ref.[13]) | - |
| $\sigma^{\#}_{\mathrm{bulk}}$ | $1\times10^{-3}$ | Ref.[9] | | | | | S/cm |
| $\sigma^{\#}_{\mathrm{total}}(\text{high }\theta)$ | $2.0\times\,10^{-4}$ | Ref.[15] | | | | | S/cm |

the conductivity becomes

$$\hat{\sigma}^{\#} = (z_+F)^2\mathscr{L}^{\#}_{++}(1-(c_+-c_0)\Delta\nu). \tag{SI-34}$$

## SI-2 Computational Details

The incompressible SE model derived in the main part of this work includes material, geometry, and experiment dependent parameters. The specification of these parameters is subject to Sec. SI-2.1. A sketch on the applied numerical methods is given in Sec. SI-2.2. In Sec. SI-2.3, we give a brief overview of how the pressure is calculated.

### SI-2.1 Parametrization

Here, we specify our standard simulation parameters. Unless indicated otherwise—e.g., in the context of parameter variations—we chose the simulation parameters as follows.

#### SI-2.1.1 Experiment Dependent Parameter

The present study focus on SEs at room temperature $\theta = 298$ K. As shown by first principles calculations[16] electrochemical potential windows of SEs are material dependent. However, with regard to the qualitative comparability of processes induced by this potential windows, we assume independent of the specific SE material an effective potential difference $U = 2V$.

#### SI-2.1.2 Geometry Parameters

We consider a SE thickness $L_{\mathrm{SE}}$ of 2400 nm corresponding to the SE layer thickness investigated in Refs.[1,2] by in situ electron holography measurements.

#### SI-2.1.3 Material Parameters

The model equations contain three kind of material parameters: transport parameters, parameters regarding the polarization response, and composition dependent parameters. The concrete material parameters used to simulate different SE materials are listed in Tab. SI-1.

- We assume the *dielectric susceptibility* $\chi_{\mathrm{SE}}$ to be independent of field variables, neglecting a possible dependence on the electric field especially in the SCLs[17]. In SEs with grain boundaries the dielectric response is strongly frequency dependent, since accumulation of charges at the

grain boundaries induce a macroscopic polarization density at low frequencies, leading to an strongly enhanced dielectric function at low frequencies (i.e., below about 1 kHz[12]). Values of the order $10^3 - 10^5$ are quite common in the quasi static response. The same accumulation of charges will occur at constant current conditions. Although, we do not simulate such an open system in this work, we would like to understand how induced effective large dielectric constants due to the creation of polarization densities at grain boundaries are affecting SCLs at the interface. Therefore, we will choose for demonstration purposes the zero frequency dielectric response for LATP and LLTO found in literature[12] although most likely this extreme limit will rarely be obtained in battery applications. A quantitative model for this current induced polarization is under investigation[18].

- Depending on the experimentally available data, the *Onsager coefficient* can be calculated from the experimentally determined conductivity $\sigma^{\#}$. In polycrystalline LLTO the experimentally determined bulk conductivity differs from the total conductivity $\sigma^{\#}_{\mathrm{total}}$ by two orders of magnitude. Matching to the zero frequency dielectric, we choose this reduced total conductivity to determine the Onsager coefficient for our transient simulation. However, this total conductivity in LLTO depends on the sintering temperature, which leads to significantly different low $\theta$ and high $\theta$ conductivities[15]. In this work, we chose the high temperature LLTO.

- The *composition dependent parameters* such as the initial concentrations are chosen such that the overall electroneutrality of the crystal is satisfied. All concentrations are normalized to the summary concentration. For reasons of comparability with Ref.[5], we consider a normalized cation site concentration of $c_v^\star = c_v/c = 0.2$.

### SI-2.2 Implementation and Numerical Methods

For the simulations, we implement our model in Matlab. All numerical examples are discretized in space by finite volume method[19], in time by implicit time stepping method and solved numerically by Newton's method globalized with Armijo-Powell-Wolfe step size rule[20–22]. To resolve the boundary layers in the SCL region numerically, the calculations are performed utilizing a grid of uniformly distributed nodes providing local grid refinements towards the boundaries.

### SI-2.3 Data Processing

The solution procedure to calculate the SE response on polarization experiments decomposes into two steps: (1) Solution of the dimensionless generalized drift-diffusion-Possion (gDDP) system. (2) Post-evaluation of pressure and current response.

Given a solution $(c,\phi)$ of the dimensionless gDDP system the elastic pressure is computed as follows. The force balance (SI-27) determines the pressure up to a constant. To calculate the elastic pressure $p = p(c,\phi)$ induced by the charge density and potential profile, further conditions are necessary. These are given by the following boundary condition on the total stress

$$\mathscr{T}\nu = \mathbf{f}, \qquad \text{on } \Gamma_i, i \in \{\mathrm{C},\mathrm{A}\}, \tag{SI-35}$$

where $\mathbf{f}$ denotes the surface force acting on the SE boundary. We suppose the surface force is given by the ambient pressure $p_0$, i.e., with $\mathbf{f} = -p_0\mathbf{I}\nu$. By means of the stress tensor (29), the pressure boundary condition (SI-35) reduces to

$$p\mathbf{I}\nu = \left(p_0\mathbf{I} - \frac{1}{2}\varepsilon_{\mathrm{SE}}|\nabla\phi|^2\mathbf{I} + \varepsilon_{\mathrm{SE}}\nabla\phi\otimes\nabla\phi\right)\nu, \qquad \text{on } \Gamma_i, i\in\{\mathrm{C},\mathrm{A}\}. \tag{SI-36}$$

In 1D, integration of the force balance together with Poisson's equation and chain rule can be used to simplify the pressure boundary condition resulting in a quadratic dependence of the boundary pressure on the electric field, respectively, on the gradient of the electro-quasi-static potential[5,23].

$$p(x) = p_0 + \frac{1}{2}\varepsilon_{\mathrm{SE}}(\partial_x\phi(x))^2, \qquad x\in\{0, L_{\mathrm{SE}}\}. \tag{SI-37}$$

## SI-3 Details on Analytical Results

This section contains the detailed derivations of the analytical results for SEs with a spatially homogeneous lattice in thermodynamic equilibrium presented in Sec. 4.1. In Sec. SI-3.1 the explicit expression for the quasi Fermi potential is derived. Sec. SI-3.2 includes the details of the approximation for low temperatures compared to the quasi Fermi potential. Finally, Sec. SI-3.3 contains the detailed derivation of the differential SCL capacity.

### SI-3.1 Derivation of the Quasi Fermi Potential

The quasi Fermi potential $\Phi$ can be calculated explicitly by evaluating the global charge neutrality condition (54) and the fact that the reduced driving force $\hat{\varphi}$ is constant in equilibrium. Combining the global charge neutrality condition (54) and Poisson's equation yields equality of the slope of $\phi$ at the boundary points

$$0 = \int_0^{L_{\mathrm{SE}}} q_F\,dx = \varepsilon_{\mathrm{SE}}\left(\partial_x\phi_L - \partial_x\phi_R\right). \tag{SI-38}$$

Multiplying the gPB equation (57) with $y(\phi(x)) = \partial_x\phi$, applying chain rule and integrating by substitution with $s := \phi(x)$ gives an expression for the electric field which basically integrates the free charge density with respect to the electric potential. The derivation of this expression further uses the setting $v = 1/2y^2$ which gives $v' = y'y$ and allows to integrate the left-hand side of the resulting equation, i.e.,

$$-\varepsilon_{\mathrm{SE}}\int \partial_{xx}\phi\,\partial_x\phi\,dx = -\varepsilon_{\mathrm{SE}}v(s) + C_{s1}, \tag{SI-39}$$

where $C_{s1}$ is an integration constant. Defined integration of Eq. (SI-39) yields

$$-\frac{\varepsilon_{\mathrm{SE}}}{2}\left[(\partial_x\phi_R)^2 - (\partial_x\phi_L)^2\right] = \int_{\phi_L}^{\phi_R} q_F(s)\,ds.$$

Linking this representation with the property (SI-38) we obtain the integral constraint

$$0 = \int_{\phi_L}^{\phi_R} q_F(s)\, ds = \frac{1}{z_+ F} \int_{\hat{\mu}_L}^{\hat{\mu}_R} q_F(u)\, du. \tag{SI-40}$$

Here the second equality follows from $s = \phi(x) = \hat{\mu}(x)/(z_+ F)$ and the substitution $u := \hat{\mu}(x)$ with the settings $\hat{\mu}_L := \hat{\mu}(0)$, $\hat{\mu}_R := \hat{\mu}(L_{\text{SE}})$ for the chemical potentials at the boundaries. Rewriting the cation concentration as a sigmoid function of the effective chemical potential and using $z_+ = -z_0$ the integral constraint (SI-40) reads

$$\int_{\hat{\mu}_L}^{\hat{\mu}_R} \left( \frac{c_1}{1 + \exp\left(-\frac{u - \hat{\mu}^\circ}{R\theta}\right)} - c_0 \right) du = 0. \tag{SI-41}$$

One the one hand, integration of the vanishing driving force condition across the SE gives the connection $\hat{\mu}_R = \hat{\mu}_L + z_+ F U$ between the reduced effective chemical potentials at the boundaries. On the other hand, integration of the integral constraint (SI-41) across the SE yields the relation

$$c_1 \ln \left( \frac{\exp\left(\frac{\hat{\mu}_R - \hat{\mu}^\circ}{R\theta}\right) + 1}{\exp\left(\frac{\hat{\mu}_L - \hat{\mu}^\circ}{R\theta}\right) + 1} \right) - c_0 (\hat{\mu}_R - \hat{\mu}_L) = 0. \tag{SI-42}$$

Combining both relations and rearranging we find the following explicit expression for the reduced effective chemical potential at the positive electrode-SE interface up to the reference chemical potential as a function of applied potential difference and composition

$$\hat{\mu}_L - \hat{\mu}^\circ = R\theta \ln \left( \frac{\exp\left(\frac{c_0}{c_1} z_+ F U\right) - 1}{\exp(z_+ F U) - \exp(\frac{c_0}{c_1} z_+ F U)} \right). \tag{SI-43}$$

Since we can characterize the constant driving force by its representation at the positive electrode-SE interface $\hat{\varphi} = \hat{\mu}_L + z_+ F U$ as well as in the bulk SE $\hat{\varphi} = \hat{\mu}_{\text{bulk}} + z_+ F \phi_{\text{bulk}}$, we arrive at explicit representations of the quasi Fermi potential and the bulk potential

$$\Phi = \frac{\hat{\mu}_L - \hat{\mu}^\circ}{z_+ F} + U, \tag{SI-44a}$$

$$\phi_{\text{bulk}} = \Phi - \frac{\hat{\mu}_{\text{bulk}} - \hat{\mu}^\circ}{z_+ F}. \tag{SI-44b}$$

Combining (SI-44a) and (SI-43) yields Eq. (59).

### SI-3.2 Approximated Generalized Poisson-Boltzmann Equation

Here we evaluate the gPB equation (57) for the low temperature approximation (61). In the charge neutral bulk region the gPB equation (57) reduces to Laplace's equation. In the SCLs the low temperature approximation results in two linear gPB equations, each of which applies in the ener-

getically different regions:

$$-\varepsilon_{\mathrm{SE}}\partial_{xx}\phi_{\mathrm{C}} = q_{\mathrm{C}}, \quad x \in [0, x_{\mathrm{C}}], \tag{SI-45a}$$

$$-\varepsilon_{\mathrm{SE}}\partial_{xx}\phi_{\mathrm{bulk}} = 0, \quad x \in [x_{\mathrm{C}}, x_{\mathrm{A}}], \tag{SI-45b}$$

$$-\varepsilon_{\mathrm{SE}}\partial_{xx}\phi_{\mathrm{A}} = q_{\mathrm{A}}, \quad x \in [x_{\mathrm{A}}, L_{\mathrm{SE}}], \tag{SI-45c}$$

where $q_{\mathrm{C}} := z_0 F c_0$ and $q_{\mathrm{A}} := z_+ F c_+^{\max} + z_0 F c_0$ are the free charge densities in the respective rectangular approximated SCLs. By integrating these linear gPBs equations (SI-45a) and (SI-45c), we obtain two potential solutions, one for each SCL

$$\phi_{\mathrm{C}}(x) = -\frac{q_{\mathrm{C}}}{2\varepsilon_{\mathrm{SE}}}x^2 + b_{1\mathrm{C}}x + b_{0\mathrm{C}}, \qquad x \in [0, x_{\mathrm{C}}], \tag{SI-46a}$$

$$\phi_{\mathrm{A}}(x) = -\frac{q_{\mathrm{A}}}{2\varepsilon_{\mathrm{SE}}}x^2 + b_{1\mathrm{A}}x + b_{0\mathrm{A}}, \qquad x \in [x_{\mathrm{A}}, L_{\mathrm{SE}}], \tag{SI-46b}$$

with four constants $b_{0i}, b_{1i}, i \in \{\mathrm{C}, \mathrm{A}\}$. We are seeking a continuous approximation of the potential throughout the SE that has the same essential characteristics as the original potential. Therefore, in addition to the boundary conditions and the equality of slopes (SI-38) at the boundaries, the potential must meet the following continuity conditions

$$\phi_{\mathrm{C}}(x_{\mathrm{C}}) = \phi_{\mathrm{A}}(x_{\mathrm{A}}) = \phi_{\mathrm{bulk}}, \tag{SI-47a}$$

$$\partial_x\phi_{\mathrm{C}}(x_{\mathrm{C}}) = \partial_x\phi_{\mathrm{A}}(x_{\mathrm{A}}) = 0. \tag{SI-47b}$$

Thus, we have seven conditions for the seven constants $b_{0i}, b_{1i}, x_i, i \in \{\mathrm{C}, \mathrm{A}\}$, and $\phi_{\mathrm{bulk}}$. The resulting non-linear expressions for the potential solution in each SCL region are:

$$\phi_{\mathrm{C}}(x) = -\frac{q_{\mathrm{C}}}{2\varepsilon_{\mathrm{SE}}}x^2 + \frac{q_{\mathrm{C}}x_{\mathrm{C}}}{\varepsilon_{\mathrm{SE}}}x + v_0, \qquad x \in [0, x_{\mathrm{C}}], \tag{SI-48a}$$

$$\phi_{\mathrm{A}}(x) = -\frac{q_{\mathrm{A}}}{2\varepsilon_{\mathrm{SE}}}x^2 + \frac{q_{\mathrm{A}}x_{\mathrm{A}}}{\varepsilon_{\mathrm{SE}}}x + \frac{q_{\mathrm{A}}L_{\mathrm{SE}}^2}{2\varepsilon_{\mathrm{SE}}} - \frac{q_{\mathrm{A}}x_{\mathrm{A}}L_{\mathrm{SE}}}{\varepsilon_{\mathrm{SE}}}, \quad x \in [x_{\mathrm{A}}, L_{\mathrm{SE}}], \tag{SI-48b}$$

with locations

$$x_{\mathrm{C}} = \sqrt{2\varepsilon_{\mathrm{SE}}U\frac{q_{\mathrm{A}}}{q_{\mathrm{C}}(q_{\mathrm{C}} - q_{\mathrm{A}})}}, \tag{SI-49a}$$

$$x_{\mathrm{A}} = \frac{q_{\mathrm{C}}x_{\mathrm{C}} + q_{\mathrm{A}}L_{\mathrm{SE}}}{q_{\mathrm{A}}}, \tag{SI-49b}$$

and bulk potential level given by

$$\phi_{\mathrm{bulk}} = U\frac{q_{\mathrm{C}}}{q_{\mathrm{C}} - q_{\mathrm{A}}}. \tag{SI-50}$$

### SI-3.3 Differential Space-Charge Layer Capacity

The differential SCL capacities $C_i$—the response of the space charge $Q_i$ to changes of the SCL potential drop $\Delta\phi_i$— is calculated via chain rule[24]

$$C_i = -\frac{dQ_i}{d\Delta\phi_i} = -\frac{dQ_i}{d\Delta p_i}\frac{d\Delta p_i}{d\Delta\phi_i}, \qquad i \in \{\text{A, C}\}, \tag{SI-51}$$

where $\Delta p_i = p_{\text{bulk}} - p_{\text{bnd}}$ denotes the SCL pressure drop. Here, the derivatives follow from the force balance (SI-27). At first, we consider the space charge given by the integrated free charge density similar to Eq. (SI-38). Since the electric field in the bulk SE vanishes, i.e., $\partial_x \phi_{\text{bulk}} = 0$, the space charge $Q_i$ is determined by the electric field at the boundary only

$$Q_i = \int_{x_{\text{bnd}}}^{x_{\text{bulk}}} q_F dx = \varepsilon_{\text{SE}} \left(\partial_x \phi_{\text{bnd}} - \partial_x \phi_{\text{bulk}}\right) = \varepsilon_{\text{SE}} \partial_x \phi_{\text{bnd}}. \tag{SI-52}$$

As a consequence of the force balance (SI-27), the electric field, in turn, depends on the root of the pressure difference

$$\partial_x \phi_{\text{bnd}} = \sqrt{\left(\partial_x \phi_{\text{bulk}}\right)^2 - \frac{2}{\varepsilon_{\text{SE}}}\left(p_{\text{bulk}} - p_{\text{bnd}}\right)} \tag{SI-53}$$

Utilizing this electric field representation then gives the SCL charge as function of pressure drop

$$Q_i(\Delta p_i) = \text{sgn}(\Delta\phi_i)\sqrt{-2\varepsilon_{\text{SE}}\Delta p_i}. \tag{SI-54}$$

Secondly, integrating the force balance (SI-27) leads to an relation between the pressure difference and the potential difference, which basically integrates the negative free charge density by substitution $s = \phi(x)$ with respect to the potential

$$\Delta p_i = -\int_{\phi_{\text{bnd}}}^{\phi_{\text{bulk}}} q_F(s)\, ds = z_+ F c_1 \ln\left(\frac{1 + \exp\left(\frac{z_+ F}{R\theta}\left(\phi_{\text{bulk}} - \Phi\right)\right)}{1 + \exp\left(\frac{z_+ F}{R\theta}\left(\phi_{\text{bnd}} - \Phi\right)\right)}\right) - F(z_+ c_1 + z_0 c_0)\Delta\phi_i. \tag{SI-55}$$

From each of these expressions follow the required derivatives

$$\frac{dQ_i}{d\Delta p_i} = -\text{sgn}(\Delta\phi_i)\sqrt{\frac{\varepsilon_{\text{SE}}}{2|\Delta p_i|}}, \qquad \frac{d\Delta p_i}{d\Delta\phi_i} = -q_F(x_{\text{bnd}}) \tag{SI-56}$$

and the general form of the differential capacity (SI-51) is given by the relation[25]

$$C_i(\Delta\phi_i) = -\text{sgn}(\Delta\phi_i)\sqrt{\frac{\varepsilon_{\text{SE}}}{2|\Delta p_i|}}\, q_{\text{bnd}}, \tag{SI-57}$$

where $q_{\text{bnd}} = q_F(x_{\text{bnd}})$ denotes the free charge density at the respective boundary, $\text{sgn}(\Delta\phi_i)$ the sign of the SCL potential drop, and $|\Delta p_i|$ the absolute value of the SCL pressure difference given by the antiderivative of the negative free charge density with respect to the SCL potential drop. For our concrete case of incompressible SEs with spatially homogeneous distributions of cations and cation

sites this results in

$$C_i(\Delta\phi_i) = -\text{sgn}(\Delta\phi_i)\sqrt{\frac{\varepsilon_{\text{SE}}}{2}}\frac{q_{\text{bnd}}}{\sqrt{F(z_+c_1+z_0c_0)\Delta\phi_i - z_+Fc_1\ln\left(\frac{1+\exp\left(\frac{z_+F}{R\theta}(\phi_{\text{bulk}}-\Phi)\right)}{1+\exp\left(\frac{z_+F}{R\theta}(\phi_{\text{bnd}}-\Phi)\right)}\right)}}. \tag{SI-58}$$

Thus, we find a non-linear analytical expression for the differential capacitance, which is a result of the material model.

## References


[1] T. Hirayama, Y. Aizawa, K. Yamamoto, T. Sato and H. Murata, *Ultramicroscopy*, 2017, **173**, 64–70.

[2] Y. Aizawa, K. Yamamoto, T. Sato, H. Murata, R. Yoshida, C. A. J. Fisher, T. Kato, Y. Iriyama and T. Hirayama, *Ultramicroscopy*, 2017, **178**, 20–26.

[3] Y. Nomura, K. Yamamoto, T. Hirayama and K. Saitoh, *Microscopy*, 2018, **67**, 178–186.

[4] A. Kovetz, *Electromagnetic Theory*, Oxford University Press, Oxford, 2006.

[5] S. Braun, C. Yada and A. Latz, *The Journal of Physical Chemistry C*, 2015, **119**, 22281–22288.

[6] R. E. Howard and A. B. Lidiard, *Reports on Progress in Physics*, 1964, **27**, 161.

[7] S. deGroot and P. Mazur, *Non-Equilibrium Thermodynamics*, North-Holland, Amsterdam, 1969.

[8] W. Dreyer, C. Guhlke and M. Landstorfer, *Electrochemistry Communications*, 2014, **43**, 75 – 78.

[9] Y. Inaguma, C. Liquan, M. Itoh, T. Nakamura, T. Uchida, H. Ikuta and M. Wakihara, *Solid State Communications*, 1993, **86**, 689 – 693.

[10] H. Jena, K. V. G. Kutty and T. R. N. Kutty, *Journal of Materials Science*, 2005, **40**, 4737–4748.

[11] S. Duluard, A. Paillassa, L. Puech, P. Vinatier, V. Turq, P. Rozier, P. Lenormand, P.-L. Taberna, P. Simon and F. Ansart, *Journal of the European Ceramic Society*, 2013, **33**, 1145 – 1153.

[12] W. Bucheli, K. Arbi, J. Sanz, D. Nuzhnyy, S. Kamba, A. Várez and R. Jimenez, *Physical chemistry chemical physics*, 2014, **16**, 15346–54.

[13] S. Larfaillou, D. Guy-Bouyssou, F. le Cras and S. Franger, *Journal of Power Sources*, 2016, **319**, 139 – 146.

[14] T. Zangina, J. Hassan, K. A. Matori, R. S. Azis, U. Ahmadu and A. See, *Results in Physics*, 2016, **6**, 719 – 725.

[15] W. J. Kwon, H. Kim, K.-N. Jung, W. Cho, S. H. Kim, J.-W. Lee and M.-S. Park, *J. Mater. Chem. A*, 2017, **5**, 6257–6262.

[16] Y. Zhu, X. He and Y. Mo, *J. Mater. Chem. A*, 2016, **4**, 3253–3266.

[17] H. Wang and L. Pilon, *Journal of Power Sources*, 2013, **221**, 252–260.

[18] A. Neumann, K. Becker-Steinberger and A. Latz, *To be published.*

[19] P. Popov, Y. Vutov, S. Margenov and O. Iliev, Numerical Methods and Applications, Berlin, Heidelberg, 2011, pp. 338–346.

[20] L. Armijo, *Pacific J. Math.*, 1966, **16**, 1–3.

[21] P. Wolfe, *SIAM Review*, 1969, **11**, 226–235.

[22] P. Wolfe, *SIAM Review*, 1971, **13**, 185–188.

[23] W. Dreyer, C. Guhlke and R. Muller, *Phys. Chem. Chem. Phys.*, 2013, **15**, 7075–7086.

[24] M. Z. Bazant, M. S. Kilic, B. D. Storey and A. Ajdari, *Advances in Colloid and Interface Science*, 2009, **152**, 48 – 88.

[25] M. Landstorfer, C. Guhlke and W. Dreyer, *Electrochimica Acta*, 2016, **201**, 187 – 219.
